# Supplementary material for: Electronic properties of linear carbon chains: resolving the controversy
Source: arXiv:1402.5812 source file (2014-02-24)
Supplement: Supplementary file 1 [file Polyyne_suppmat_17-2-14.pdf]

# Supplementary Material: Electronic properties of linear carbon chains: resolving the controversy.

Amaal Al-Backri[1,2], Viktor Zólyomi[1], and Colin J. Lambert[1]
[1]*Physics Department, Lancaster University, LA1 4YB, Lancaster United Kingdom and*
[2]*Baghdad University, College of Science,Al-Jaderyia campus, Baghdad, Iraq*

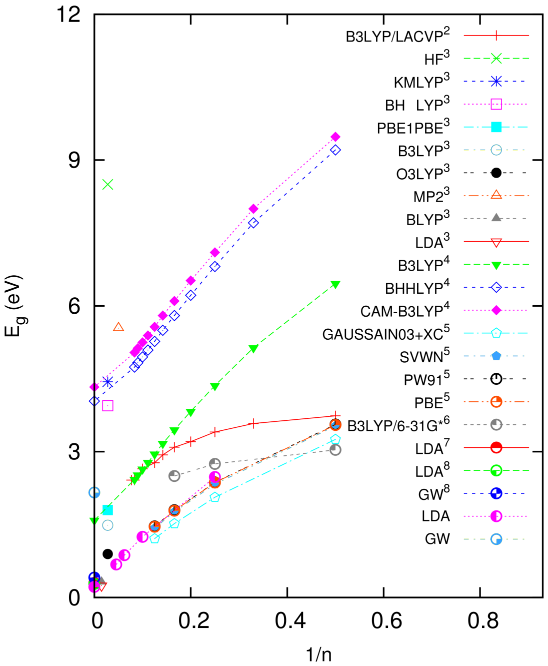


Figure S.1. Theoretical values of the HOMO-LUMO gap ($E_g$) of oligoynes and polyyne as a function of $1/n$ (where n equals the number of carbon pairs) using various methods. The last two items of data correspond to our own results using LDA in the SIESTA code and GW in VASP.

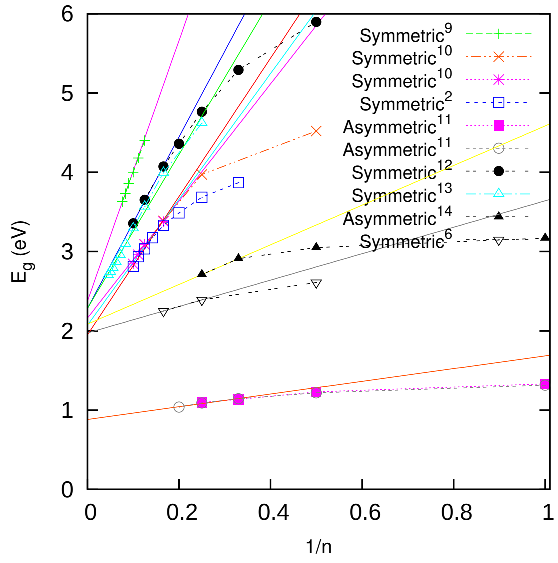


Figure S.2. Experimental values of the HOMO-LUMO gap of short oligoynes as a function of $1/n$ (where n equals the number of carbon pairs) of different molecules terminated with symmetric and asymmetric arrangements of end groups. Linear extrapolation to the limit of infinite oligoyne length estimates the band gap of polyyne between 2.0 and 2.3 eV in the majority of these measurements which is in excellent agreement with our GW results.

We begin by presenting a range of theoretical and experimental values for the HOMO-LUMO gaps of finite oligoynes and extrapolate these to infinitely-long chains to obtain estimates of the band gap $E_g$ of an infinite polyyne. To demonstrate the wide range of inconsistent theoretical predictions for $E_g$, Figure S.1 shows a summary of existing values. To demonstrate the range of experimental values for $E_g$, Figure S.2 shows a summary of existing literature values.

To illustrate the inadequacy of DFT, we performed calculations using the local density approximation (LDA) within the SIESTA code [1]. Both infinite polyyne and short oligoyne chains were analyzed. A double zeta polarized (DZP) basis set was used and the force tolerance on the atoms was set to a strict 0.00005 eV/Å.

Short oligoynes were examined up to a length of 44 carbon atoms. The end groups were modelled after a recent experiment [13] for easy comparison; their structure is illustrated in Figure S.3. These molecules were also studied in a DZP basis but with a more lenient force tolerance of 0.01 eV/Å due to the number of atoms involved. Unsurprisingly, their HOMO-LUMO gap is significantly below the measured data (see Figure S.2). For the case of an infinitely-periodic polyyne, we found a band gap of 0.2 eV which is in good agreement with previous LDA calculations which predicted 0.3 eV using a superior plane-wave basis description [7]. These results are plotted in Figure S.1.

The HSE06 and GW calculations on an infinitely periodic polyyne, with two carbon atoms per unit cell, were performed using the VASP code [15, 16]. The plane-wave cutoff energy was set to 420 eV and the artificial separation of the polyyne chains in the three-dimensional unit cell was 10 Å. The HSE06 calculations were performed with increasing density of $k$-points until convergence was reached at a Γ centered Monkhorst-Pack grid of $1\times1\times30$.

The GW calculations were done using the same set of $k$-points in the optimized HSE06 geometry with the single shot G0W0 approach. The wave functions of the

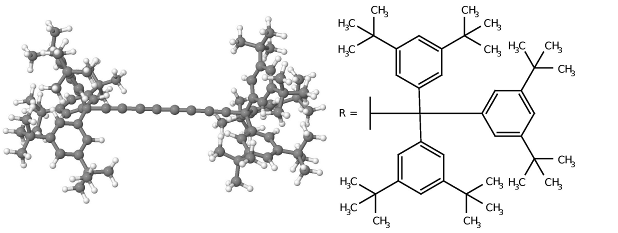


Figure S.3. Example of the relaxed structure of the short oligoynes in this study (left) and the sketch of their end groups (right). This end group was used in recent experiments [13].

HSE06 method were used as a starting point. The spectral method was applied calculating the imaginary part of the independent particle polarizibility first, followed by a Kramers-Kronig transform to obtain the full polarizibility. This calculation depends quite strongly on $N_b$, the number of bands. Convergence in $N_b$ was reached at $N_b = 180$. $N_\omega$, the number of frequency points used in the integration of the response function by the spectral method, was set to 48. Figure S.4 illustrates the convergence of the band gap as the number of bands $N_b$ is increased.

Note that the single-shot GW approximation depends heavily on the starting wave function, see e.g. [17, 18]. The HSE wave functions are widely considered an optimal choice which is why we used them. However, in order to estimate the uncertainty in the gap arisen from the use of single-shot GW, we performed a fully self- consistent GW calculation with the same parameters that we used to calculate the single-shot GW band structure in Fig. 1. We have found that the band gap is reduced to 2.15 eV which is a very small change and illustrates that for polyyne the HSE wave functions are indeed an excellent starting point for single-shot GW calculations.

The analytical formula for the $\beta$-value as a function of energy was derived using a nearest neighbor one electron per site tight-binding (TB) model. The structure consists of two sublattices; their wave functions can be denoted as $\psi_j$ and $\phi_j$ as shown in Figure S.5. The on-site energy is $\varepsilon_c$ and $\alpha$ and $\gamma$ denote the alternating couplings between neighbourig atoms connected by short and long bonds, respectively.

The Schrödinger equation takes the form

$$\varepsilon_c \psi_j - \alpha \phi_j - \gamma \phi_{j-1} = E \psi_j, \tag{1}$$

$$\varepsilon_c \phi_j - \alpha \psi_j - \gamma \psi_{j+1} = E \phi_j, \tag{2}$$

and can by solved by inserting Bloch wavefunctions

$$\psi_j = A \cdot e^{ikaj}, \phi_j = B \cdot e^{ikaj} \tag{3}$$

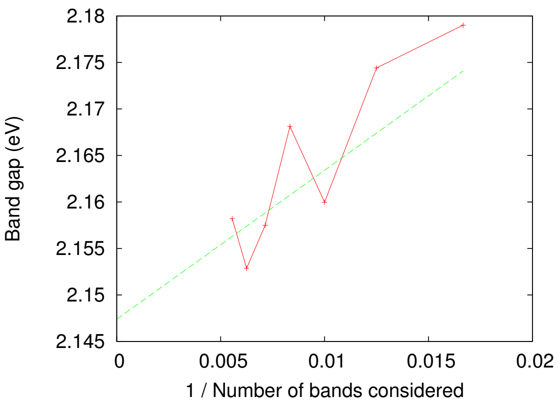


Figure S.4. Variation of the band gap with $1/N_b$, where $N_b$ is the number of bands used in the G0W0 calculation.

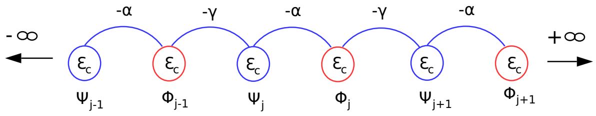


Figure S.5. The model of alternating coupling in a one-dimensional linear carbon chain (see text).

where $A$ and $B$ are constants, $a$ is the lattice constant and $k$ is the wave vector. By substituting equation 3 into equations 1 and 2 we find

$$\varepsilon_c \cdot A - \Delta(-k) \cdot B = E \cdot A, \tag{4}$$

$$\varepsilon_c \cdot B - \Delta(k) \cdot A = E \cdot B, \tag{5}$$

where $\Delta(k) = \alpha + \gamma \cdot e^{ika}$. Therefore the Hamiltonian takes the following form:

$$H = \begin{pmatrix} \varepsilon_C & -\Delta(-k) \\ -\Delta(k) & \varepsilon_C \end{pmatrix}. \tag{6}$$

Diagonalization yields

$$E - \varepsilon_c = \pm\sqrt{\alpha^2 + \gamma^2 + 2\alpha\gamma \cos ka(E)} \tag{7}$$

$$\cos ka(E) = \Theta(E), \tag{8}$$

where $\Theta(E) = ((\varepsilon_c - E)^2 - (\alpha^2 + \gamma^2))/2\alpha\gamma$.

Using $\cos ka = \frac{e^{ika} + e^{-ika}}{2}$ yields

$$e^{ika} = \Theta(E) \pm \sqrt{(\Theta(E))^2 - 1}. \tag{9}$$

The solution depends on the sign of the expression under the square root. If $|\Theta(E)| < 1$ then $ka(E)$ is real,

while if $|\Theta(E)| > 1$ then $ka(E)$ is complex and we define the attenuation factor $\beta$ by

$$\beta = \frac{2\mathrm{Im}(ka(E))}{a} = \frac{-2\ln[|\Theta(E)| - \sqrt{\Theta^2(E) - 1}]}{a}. \quad (10)$$

For energies within the band, fitting equation (7) to our GW band structure yields $\gamma$=4.657 eV and $\alpha$=3.548 eV. The maximum of $\beta$ is attained when $E - (\varepsilon_c = 0$, in which case

$$\Theta = \frac{-\alpha^2 - \gamma^2}{2\alpha\gamma} = -1.0372, \quad (11)$$

and $\beta$ achieves a maximum value of $\beta_{max} = 0.21$ Å$^{-1}$.

---


[1] Soler,J. M. and Artacho, E. and Galea,J. D. and Garcia, A. and Junquera, J. and Ordejón, P. and Sánchez- Portal, D. J. , Phys. Condens. Matter 2002, 14, 2745.

[2] Zhuravlev, F. and Gladysz, J. A., Chemistry-A European Journal, 10, 24, 6510 2004.

[3] Yang, S. and Kertesz, M., J. Phys. Chem. A, 2006, 110, 9771.

[4] Peach, M. J.and Tellgren, E. I.and Salek, P. and Helgaker, T. and Tozer, D. J., J. Phys. Chem. A, 2007, 111, 11930.

[5] Crljen,Ž.and Baranović, G. Phys. Rev. Lett. 2007, 98, 116801.

[6] Chen, G. and Mahmud, I. and Dawe, L. N.and Daniels, L. M. and Zhao, Y., J. Org Chem., 2011, 76, 2701.

[7] Rusznyák, Á. and Zólyomi, V. and Kürti, J. and Yang, S. and Kertesz, M., Phys. Rev. 2005, B72 155420.

[8] Cretu,O. and Botello-Mendez,A. R.and Janowska,I. and Pham-Huu, C.and Charlier, J.-C. and Banhart,F. , arXiv:1302.5207

[9] Pino, T. and Ding, H. and Güthe, F.,and Maier, J. P., J. Chem. Phys. 2001, 114, 2208.

[10] Gibtner, T. and Hampel, F. and Gisselbrecht, J.-P. and Hirsch, A., Chemistry-A European Journal 2002, 8, 408.

[11] Xu, G.-L. and Wang, C.-Y. and Ni, Y.-H. and Goodson, T. G. and Ren, T., Organometallics, 2005, 24, 3247.

[12] Eisler, S. and Slepkov, A. D. and Elliott, E. and Luu, T. and McDonald, R. and Hegmann, F. A. and Tykwinski, R. R., JACS 2005,127, 2666

[13] Chalifoux, W. À.and Tykwinski, R. R. Nat. Chem. 2010, 2, 967-971.

[14] Pålsson, L.-O. and Wang, C. and Batsanov, À. S. and King, S. M. and Beeby, À. and Monkman, À. P. and Bryce, M. R., Chemistry-À European Journal, 2010, 16, 1470.

[15] Kresse,G. and Hafner,J., Phys. Rev. B 1993, 48, 13115.

[16] Kresse,G.and Furthmüller, J., Comput. Mater. Sci. 1996, 6, 15.

[17] Tran,F. and Blaha,P., Phys. Rev. Lett. 2009, 102, 226401.

[18] Waroquiers,D., Lherbier,A., Miglio,A., Stankovski,M., PoncÃ©,S., Oliveira2,M.J.T., Giantomassi,M., Rignanese,G.M., and Gonze,X., Phys. Rev. B 2013, 87, 075121.
